# Supplementary material for: Diffusion probabilistic modeling of protein backbones in 3D for the motif-scaffolding problem
Source: arXiv:2206.04119 source file (2023-03-20)
Supplement: Supplementary file 1 [file additional_model_samples.tex]

\begin{figure}
\includegraphics[width=1.0\textwidth]{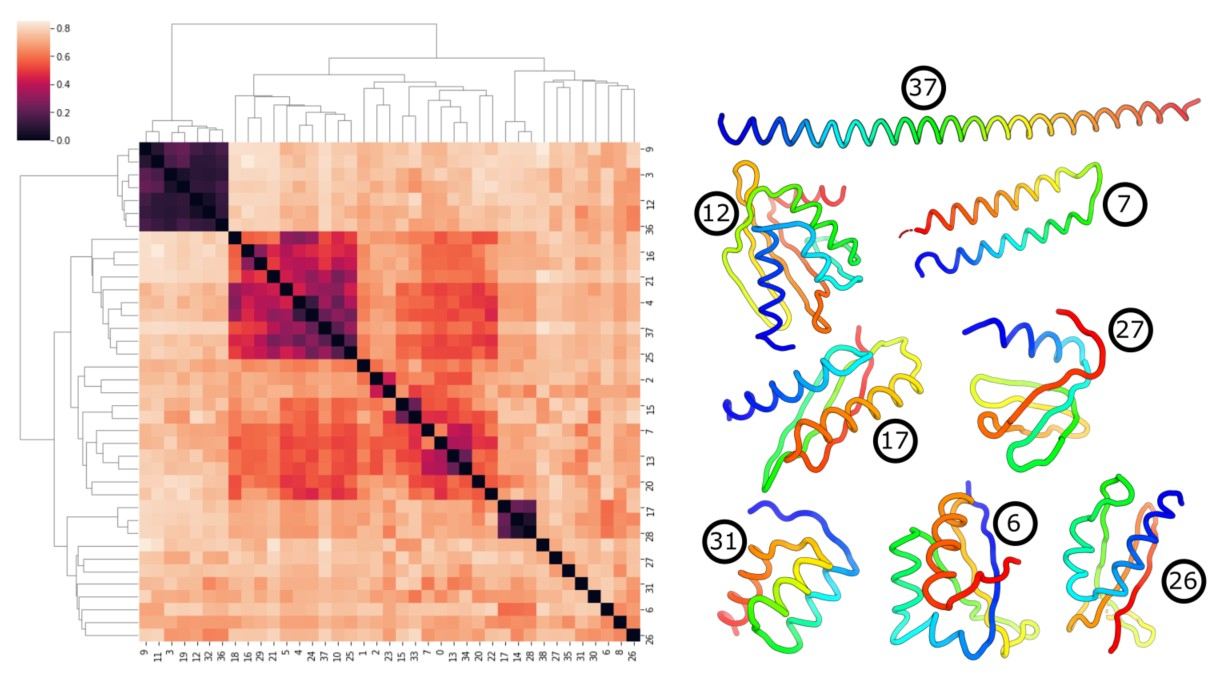}
\caption{
Structural clustering of model samples with scRMSD <2$\AA$.
(Left) hierarchical clustering on \texttt{TMScore}.
(Right) cluster centroids (defined as the sample with the smallest maximum distance to other cluster members.  \BLT{Check with Doug that this is correct}.
}\label{fig:structural_clustering}
\end{figure}
